# Supplementary material for: Uncertainty Quantification for Nuclear Density Functional Theory and Information Content of New Measurements
Source: arXiv:1501.03572 source file (2015-01-15)
Supplement: Supplementary file 1 [file uq_nuclear_dft_supp.pdf]

# Uncertainty Quantification for Nuclear Density Functional Theory and Information Content of New Measurements

J.D. McDonnell,[1,2] N. Schunck,[2] D. Higdon,[3] J. Sarich,[4] S.M. Wild,[4] and W. Nazarewicz[5,6,7]

[1] *Department of Physics and Astronomy, Francis Marion University, Florence, South Carolina 29501, USA*
[2] *Physics Division, Lawrence Livermore National Laboratory, Livermore, California 94551, USA*
[3] *Los Alamos National Laboratory, Los Alamos, New Mexico 87545, USA*
[4] *Mathematics and Computer Science Division, Argonne National Laboratory, Argonne, Illinois 60439, USA*
[5] *Department of Physics and Astronomy and NSCL/FRIB Laboratory, Michigan State University, East Lansing, Michigan 48824, USA*
[6] *Physics Division, Oak Ridge National Laboratory, Oak Ridge, Tennessee 37831, USA*
[7] *Institute of Theoretical Physics, Faculty of Physics, University of Warsaw, Warsaw, Poland*

(Dated: January 12, 2015)

## Experimental datasets

The experimental dataset of UNEDF1 contains $n_d = 115$ data points [1, 2], which can be broken down into $n_T = 4$ data types: $n_1 = 75$ nuclear masses (28 spherical and 47 deformed), $n_2 = 28$ r.m.s. proton radii, $n_3 = 8$ odd-even mass staggering differences (4 for neutrons and 4 for protons), and $n_4 = 4$ excitation energies of fission isomers. Compared with UNEDF1, the UNEDF1$_{\mathrm{CPT}}$ dataset contains 17 new masses of neutron-rich even-even nuclei measured by using the Canadian Penning Trap mass spectrometer and CARIBU facility [3–5] at Argonne National Laboratory. These new data are listed in Table I.

TABLE I. Experimental binding energies (rounded to the nearest 0.1 MeV) of the 17 even-even nuclei measured in Refs. [3–5] included in our analysis.

| Nucleus | $B$ (MeV) | Ref. |
|---|---|---|
| $^{130}$Sn | -1090.2 | [5] |
| $^{132}$Sn | -1102.7 | [5] |
| $^{134}$Sn | -1108.8 | [5] |
| $^{134}$Te | -1123.3 | [4] |
| $^{136}$Te | -1131.3 | [4] |
| $^{138}$Te | -1138.7 | [5] |
| $^{140}$Te | -1145.7 | [5] |
| $^{138}$Xe | -1151.4 | [4] |
| $^{140}$Xe | -1160.6 | [4] |
| $^{142}$Ba | -1180.0 | [3] |
| $^{144}$Ba | -1190.1 | [3] |
| $^{146}$Ba | -1199.4 | [3] |
| $^{146}$Ce | -1208.5 | [3] |
| $^{148}$Ce | -1219.4 | [3] |
| $^{150}$Ce | -1230.0 | [3] |
| $^{158}$Sm | -1291.8 | [4] |
| $^{160}$Sm | -1302.9 | [4] |

## UNEDF coupling constants

Table II lists the coupling constants of the UNEDF0 [1], UNEDF1 [2], and UNEDF1$_{\mathrm{CPT}}$ (this work) energy density functionals.

TABLE II. Coupling constants of the UNEDF0, UNEDF1, and UNEDF1$_{\mathrm{CPT}}$ energy density functionals. $\rho_{\mathrm{c}}$ is in fm$^{-3}$; $E^{\mathrm{NM}}/A$, $K^{\mathrm{NM}}$, $a^{\mathrm{NM}}_{\mathrm{sym}}$, and $L^{\mathrm{NM}}_{\mathrm{sym}}$ are in MeV; $1/M^*_s$ is dimensionless; $C^{\rho\Delta\rho}_t$ and $C^{\rho\nabla J}_t$ are in MeV fm$^5$; and $V^n_0$ and $V^p_0$ are in MeV fm$^3$.

| Name | UNEDF0 | UNEDF1 | UNEDF1$_{\mathrm{CPT}}$ |
|---|---|---|---|
| $\rho_{\mathrm{c}}$ | 0.1605 | 0.1587 | 0.1589 |
| $E^{\mathrm{NM}}/A$ | -16.0559 | -15.8000 | -15.8000 |
| $K^{\mathrm{NM}}$ | 230.0000 | 220.0000 | 220.0000 |
| $a^{\mathrm{NM}}_{\mathrm{sym}}$ | 30.5429 | 28.9362 | 29.3449 |
| $L^{\mathrm{NM}}_{\mathrm{sym}}$ | 45.0804 | 40.0149 | 40.7144 |
| $1/M^*_s$ | 0.9000 | 0.9924 | 0.9686 |
| $C^{\rho\Delta\rho}_0$ | -55.2606 | -45.1289 | -43.9801 |
| $C^{\rho\Delta\rho}_1$ | -55.6226 | -145.3178 | -114.2915 |
| $V^n_0$ | -170.3740 | -186.0655 | -182.2372 |
| $V^p_0$ | -199.2020 | -206.5796 | -203.9807 |
| $C^{\rho\nabla J}_0$ | -79.5308 | -74.0264 | -72.4172 |
| $C^{\rho\nabla J}_1$ | 45.6302 | -35.6584 | -32.9206 |

[1] M. Kortelainen, T. Lesinski, J. Moré, W. Nazarewicz, J. Sarich, N. Schunck, M. V. Stoitsov, and S. Wild, Phys. Rev. C **82**, 024313 (2010).

[2] M. Kortelainen, J. McDonnell, W. Nazarewicz, P. Reinhard, J. Sarich, N. Schunck, M. V. Stoitsov, and S. M. Wild, Phys. Rev. C **85**, 024304 (2012).

[3] G. Savard, J. Wang, K. Sharma, H. Sharma, J. Clark, C. Boudreau, F. Buchinger, J. Crawford, J. Greene, S. Gulick, A. Hecht, J. Lee, A. Levand, N. Scielzo, W. Trimble, J. Vaz, and B. Zabransky, Int. J. Mass Spectrom. **251**, 252 (2006).

[4] J. Van Schelt, D. Lascar, G. Savard, J. A. Clark, S. Caldwell, A. Chaudhuri, J. Fallis, J. P. Greene, A. F. Levand, G. Li, K. S. Sharma, M. G. Sternberg, T. Sun, and B. J. Zabransky, Phys. Rev. C **85**, 045805 (2012).

[5] J. Van Schelt, D. Lascar, G. Savard, J. A. Clark, P. F. Bertone, S. Caldwell, A. Chaudhuri, A. F. Levand, G. Li, G. E. Morgan, R. Orford, R. E. Segel, K. S. Sharma, and M. G. Sternberg, Phys. Rev. Lett. **111**, 061102 (2013).
